# Supplementary material for: PRANK: a singular value based noise filtering of multiple response datasets for experimental dynamics
Source: arXiv:2405.07578 source file (2024-07-23)
Supplement: Supplementary file 1 [file appendix.tex]

% !TeX spellcheck = en_US

%\section{Gradient-based displacement identification}
%\label{sec:APP_1}
%This section provides a short derivation of the optical flow technique used in this work to estimate displacement from camera images. \\ 
%Assume small displacements $\Delta x$ and $\Delta y$ between two frames of an image sequence and consider negligible the change in image intensity of the same observed part of the system. The basic optical flow equations can be derived on a first order approximation as:
%\begin{equation}
%\label{eq:OF}
%\frac{\partial I_i}{\partial x}\Delta x+\frac{\partial I_i}{\partial y}\Delta y+\Delta I_i(x,y)=0
%\end{equation}
%where $\frac{\partial I_i}{\partial x}$, $\frac{\partial I_i}{\partial y}$ are the intensity gradient in $x$ and $y$, $\Delta I_i(x,y)=\frac{\partial I_i}{\partial t}\Delta t$ is the change of intensity between two consecutive frames and ${()}_i$ denotes the observed pixel. \\
%For a single pixel, the above equation results in an under-determined problem to solve for the two unknowns $\Delta x$ and $\Delta y$. However, the displacement orthogonal to the gradient vector is accessible. So, e.g. for an horizontal edge, $\frac{\partial I_i}{\partial x}=0$ and $\Delta y$ can be computed as:
%\begin{equation}
%\label{eq:SGOF}
%\Delta y=\frac{-\Delta I_i(x,y)}{\frac{\partial I_i}{\partial y}}
%\end{equation}
%The same is valid for a vertical edge and the estimation of displacement in $x$ direction.\\
%The sensitivity to displacement identification strongly depends on the spatial intensity gradient. Hence, speckle patterns or grids are commonly adopted to guarantee an adequate contrast for the measured surface.
%
%\section{Modal identification} 
%\label{sec:APP_2}
%A concise mathematical insight into the modal identification approach used in this work is hereby presented.\\ 
%A single-reference Least-Square Complex Frequency (LSCF) algorithm is used to estimate the complex eigenvalues according to:
%\begin{equation}
%\label{eq:Lambda}
%\mathbf{\lambda}_n=-\mathbf{\zeta}_n\mathbf{\omega}_n\pm i\mathbf{\omega}_n\sqrt{1-\mathbf{\zeta}_n}
%\end{equation}
%where $\mathbf{\omega}_n$ are the natural eigenfrequencies $\mathbf{\omega}_n$ and $\mathbf{\zeta}_n$ the modal damping ratios. \\
%The mode shapes are then estimated by a best fit of a mode superposition following the Least-Square Frequency Domain formulation (LSFD):
%\begin{equation}
%\label{eq:LSFD}
%\mathbf{Y}_{oi}(\omega)=\sum_{n=1}^{N}\left(\dfrac{\prescript{}{n}{\mathbf{A}_{jk}}}{i\omega-\mathbf{\lambda}_r}+\dfrac{\prescript{}{n}{\mathbf{A}_{jk}^*}}{i\omega-\mathbf{\lambda}_r^*}\right)- \dfrac{\mathbf{A}_L}{\omega^2}+ \mathbf{A}_U
%\end{equation}
%where $\prescript{}{n}{\mathbf{A}_{jk}}$ are the modal constants, $\mathbf{A}_U$ and $\mathbf{A}_L$ the upper and lower residuals and $\mathbf{Y}_{oi}$ denotes the FRFs measured in $o$ due to an excitation in $i$.\\
%
%
%\section{Stabilization diagrams for the experimental modal analysis application} 
%\label{sec:APP_3}
%In this short section, the comparison between the stabilization diagrams for poles identification on the available datasets analyzed in \cref{subsec:EE_3} is provided. The charts are offered by pyEMA. The three cases covered in \cref{fig:stabilization} compare raw camera data, filtered camera data and reference accelerometer data. The stabilization shows the sum of all FRFs included in the given dataset. In the case of the accelerometer, a single FRF is used to estimate the poles, thus explaining the shape of the curve with respect to the other two. Stable poles are clearly identified within the frequency range of interest only from accelerometer data and filtered camera data.
%
%\begin{figure} 
%	\centering
%	\begin{subfigure}{1\textwidth}
%		\centering
%		\includegraphics[width=1\linewidth]{pole_chart_1.png}
%	\end{subfigure}
%	\begin{subfigure}{1\textwidth}
%	\centering
%	\includegraphics[width=1\linewidth]{pole_chart_2.png}
%\end{subfigure}
%	\begin{subfigure}{1\textwidth}
%	\centering
%	\includegraphics[width=1\linewidth]{pole_chart_3.png}
%\end{subfigure}
%	\caption{Stabilization diagrams for poles identification within single-reference LSCF. Images provided by PyEMA. Top: Raw camera data. Center: Accelerometer data. Bottom: $PRANK_{HiP}$ camera data.}
%	\label{fig:stabilization}
%\end{figure}
